# Supplementary material for: Interim Report on Human-Guided Adaptive Hyperparameter Optimization with Multi-Fidelity Sprints
Source: arXiv:2505.09792 source file (2025-05-14)
Supplement: Supplementary file 1 [file 12A_AdditionalCapabilities.tex]

In addition to the above capabilities, which have been implemented or are under development, the following list includes additional extensions under consideration.

\begin{description}
\item[Finetuning Strategy:] %DeBERTa-v3?
    Early finetuning runs through the pre-trained transformer with randomly initialized heads for the four tasks risks being destructive to lower layers of the model. A better fine-tuning strategy may entail a training protocol that initially freezes the transformer and then enables certain layer combinations to receive gradients as training progresses.
    \item[LoRA for MTL:] Low-Rank Adaptation (LoRA) is mostly considered a parameter-efficient fine-tuning method. It can also decouple incompatible task objectives back-propagating conflicting gradient updates in a multi-task setting. This can be achieved by freezing the shared encoder transformer and establishing different LoRA states for each competing task.
    \item[Meta-Learning:] Our current approach uses a simple meta-learner that calibrates thresholds for evaluation only. Can we find a way to efficiently use meta-learning techniques for training we may be able to generalize better and automate the tuning of additional hyperparameters? 
    \item[Data Imbalance:] Evaluate if weighting relation classification task losses (or their gradients) by class frequency improves performance and contributes to resolving the effects of class imbalance in the training dataset.
    \item[Coding Fixes:] We need to (1) complete some of the changes that are currently only applied to the joint model to also work with the single-objective models. (2) Rerun experiments and compile analysis. (3) Address discretionary items, such as compiling the model under PyTorch 2, which currently fails. (4) Cleanup code and publish the paper (at least part 1.)  
    
\end{description}
