# Supplementary material for: Interim Report on Human-Guided Adaptive Hyperparameter Optimization with Multi-Fidelity Sprints
Source: arXiv:2505.09792 source file (2025-05-14)
Supplement: Supplementary file 2 [file A0A_Appendix1.tex]

\subsection{POS, MTL, ASL Options}
% \begin{table}
% \footnotesize
% \input{compPosMtsAsl.tex}
% \caption{Statistics from five training runs for all combinations of Part-of-Speach (POS), Dynamic multi-task weights (MTL), and Asymmetric losses (ASL)}
% \label{tab:posmtlaslcomp}
% \end{table}

The three options described below. We then used the best model from each run to calculate the mean and standard deviation of the five relation F1 micro scores. Relations are deemed correct if their category and the types of the associated entities match the golden truth.  \autoref{tab:posmtlaslcomp} shows these statistics for each combination of the three options below: 
\begin{description}
\item [Part of Speech (POS)] uses the tokenizer and parser from Spacy (release 3.3.1.) and aligns the token sequences with those from the Bert tokenizer. It then extracts the \emph{pos} linguistic feature of each Spacy token which it encodes and maps to a POS embedding that is appended to the output of the \emph{bert-base-cased encoder} \cite{DBLP:journals/corr/abs-1810-04805}. The resulting extended encoding is used in all input representations. 
\item [Dynamic Multi-Task Loss Balancing (MTL)] uses the method described in \autoref{sec:MTLuncert}. We use Shanon’s entropy for sampling uncertainty, and $\lambda = 0.01$ in \autoref{eq:uncertLoss}. 
\item [Asymmetric Task Loss (ASL)] is a task-level method of adjusting loss weights described in \autoref{sec:ASL}. We use probability shift $m=0.01$, positive focusing parameter $\gamma^+=1$ and negative focusing parameter $\gamma^- =2$
\end{description}
